# Supplementary material for: Magnetic-Field Dependence of Tunnel Couplings in Carbon Nanotube Quantum Dots
Source: arXiv:1204.6718 source file (2012-05-01)
Supplement: Supplementary file 1 [file SM.pdf]

# Magnetic field dependence of tunnel couplings in carbon nanotube quantum dots
# Supplemental Material

K. Grove-Rasmussen, S. Grap, J. Paaske, K. Flensberg,
S. Andergassen, V. Meden, H. I. Jørgensen,
K. Muraki, and T. Fujisawa

## Tunnel-coupling asymmetry - the spinless single-shell model

Here we present more details of the model that we use to understand aspects of the strong and weak coupling behavior as well as the $B_{||}$ dependence of the level positions. Since these effects are due to the orbital degree of freedom, we ignore the spin degree of freedom.

For a clean tube there are two degenerate quantum dot states, corresponding to the $K$ and $K'$ valleys and we denote these by $|K\rangle$ and $|K'\rangle$. For a smooth confinement potential the wave functions have the form[1, 2]

$$\langle \mathrm{r}|K^\tau\rangle = e^{i(\mathbf{K}^\tau\cdot\mathbf{C})\theta/2\pi} e^{ik_c R\theta} f(x)\mathbf{X}^\tau, \tag{1}$$

where $\tau = \pm 1$ denotes the two $K$ and $K'$ points, $\mathbf{C}$ is the chiral vector, $\theta$ the azimuthal angle, and $k_c$ describes the subband and nanotube type. Furthermore $f$ is an envelope function, $x$ the coordinate along the tube, and $\mathbf{X}^\tau$ the spinor with the two elements describing the weight of the wavefunction on the $A$ and $B$ sublattices. For metallic (or small bandgap tubes), $k_c = 0$ and

$$e^{i\mathbf{K}^\tau\cdot\mathbf{C}} = e^{i2\pi\tau(n_1-n_2)/3}. \tag{2}$$

We can therefore write the angular part of the wavefunctions as

$$\phi_K(\theta) = \langle\theta|K\rangle = \frac{1}{\sqrt{2\pi}}e^{iq\theta}, \quad \phi_{K'}(\theta) = \langle\theta|K'\rangle = \frac{1}{\sqrt{2\pi}}e^{-iq\theta}, \tag{3}$$

where the orbital quantum number $q$ is given by $q = (n_1 - n_2)/3$, which is always an integer for a metallic tube. Here $n_1$ and $n_2$ are the chiral vector indexes. For an armchair nanotube $n_1 = n_2$ and there is hence no difference in the oscillating part of the wavefunction. For all other tubes, the two states are characterized by plane waves running in opposite directions. The two states are time-reversed partners and the respective tunnel couplings to the leads are

therefore equal $|t_K| = |t_{K'}| = t$. To be more specific, $t_{\nu K} = t^*_{\overline{\nu} K'}$, where $|\nu\rangle$ and $|\overline{\nu}\rangle$ are time-reversed partner states in the leads. For simplicity, we assume these amplitudes to be independent of $\nu$.

Applying a magnetic field along the axis of the cylinder increases (lowers) the energy of $|K\rangle$ ($|K'\rangle$), *i.e.*, $\epsilon_K = B_{||}$ and $\epsilon_{K'} = -B_{||}$ (setting $\mu_{\mathrm{orb}} = g_{\mathrm{orb}}\mu_B = 1$). We also consider an intra-shell orbital coupling $|\Delta_{KK'}|e^{i\phi_0}$ with phase $\phi_0$, which couples the two states[1]. The Hamiltonian in the basis $\{|K\rangle, |K'\rangle\}$ thus becomes

$$H = \begin{bmatrix} B_{||} & \frac{|\Delta_{KK'}|}{2}e^{i\phi_0} \\ \frac{|\Delta_{KK'}|}{2}e^{-i\phi_0} & -B_{||} \end{bmatrix}, \tag{4}$$

which has eigenenergies

$$\epsilon_{b/a} = \pm\epsilon_0, \quad \epsilon_0 = \frac{1}{2}\sqrt{\left(4B_{||}^2 + \Delta_{KK'}^2\right)}, \tag{5}$$

and corresponding eigenstates

$$|b\rangle = -ve^{i\phi_0}|K\rangle + u|K'\rangle, \qquad |a\rangle = ue^{i\phi_0}|K\rangle + v|K'\rangle, \tag{6}$$

where $u$ and $v$ are (real) functions of the magnetic field:

$$(u,v) = \sqrt{\frac{1}{2}\left(1 \pm \frac{B_{||}}{\epsilon_0}\right)}. \tag{7}$$

In the simple case of $B_{||} = 0$, the two states reduce to

$$|b\rangle = \frac{1}{\sqrt{2}}(-e^{i\phi_0}|K\rangle + |K'\rangle), \quad |a\rangle = \frac{1}{\sqrt{2}}(e^{i\phi_0}|K\rangle + |K'\rangle). \tag{8}$$

In general the system is coupled to a left and a right lead in a quantum dot configuration. The tunneling hamiltonian for one lead is

$$H_t = \sum_{k_L}(t_K c^\dagger_{k_L} c_K + t_{K'} c^\dagger_{k_L} c_{K'} + \mathrm{H.c.}). \tag{9}$$

Considering only a specific $k_L$ for simplicity, the effective tunnel coupling into the $b$ state becomes (absorbing phase factors of $t_K$ and $t_{K'}$ into the unknown phase $\phi_0$)

$$|t_b(B_{||} = 0)|^2 = |\langle k_L|H_L|b\rangle|^2 = 2t^2\sin^2(\phi_0/2), \tag{10}$$

and, similarly, for the $a$ state

$$|t_a(B_{||} = 0)|^2 = 2t^2\cos^2(\phi_0/2). \tag{11}$$

The tunnel coupling to the two eigenstates therefore depends on the phase of the orbital coupling and for $\phi_0 = \pi$ the result shown in the Letter is obtained (Fig.

[1] The intra-shell orbital coupling results from a matrix element due to an impurity potential and therefore generally has a nontrivial phase.

1(e)). For finite field, the tunneling matrix elements for a general superposition $|c\rangle = x|K\rangle + y|K'\rangle$ become $|t_c|^2 = |\langle k_L|H_L(x|K\rangle + y|K'\rangle)|^2 = t^2(|x|^2 + |y|^2 + 2\mathrm{Re}\, xy^*)$, which for the two states $a$ and $b$ becomes

$$|t_{a,b}|^2 = t^2 \left[1 \pm \frac{|\Delta_{KK'}|^2}{B_{||}^2 + |\Delta_{KK'}|^2} \cos(\phi_0)\right] \tag{12}$$

Next, we examine the probability distribution (electron density) of an electron around the nanotube circumference (angle $\theta$). The electron density for the two states at $B_{||} = 0$ becomes

$$|\phi_b(\theta)|^2 = |\langle\theta|b\rangle|^2 = \frac{1}{\pi}\sin^2(q\theta + \frac{\phi_0}{2}) \tag{13}$$

$$|\phi_a(\theta)|^2 = |\langle\theta|a\rangle|^2 = \frac{1}{\pi}\cos^2(q\theta + \frac{\phi_0}{2}) \tag{14}$$

which represent two standing waves around the circumference. Here the maxima of the electron densities are shifted along $\theta$ as the phase of the orbital coupling is increased and in the article the electron density is shown for the orbital quantum number $q = 5$. Note, that this number depends on the chirality of the nanotube. The important point is that tunneling into these states is different, and therefore can explain the observed difference in tunnel coupling. As $B_{||}$ increases the prefactors $(u, v) \to (1, 0)$ according to Eq. (7), and the original plane wave states are gradually obtained (Eq. (3)) as depicted in Fig. 1(g).

As pointed out in the Letter, the model does not take into account first tunneling into a lead nanotube segment and then into the contact. This approach is hard to model, since it is difficult to imagine that the orbital coupling in the nanotube lead segment will be the same as in the quantum dot. In fact, the different orbital wave functions in the quantum dot (see Fig. 1(f)) imply that the tunnel amplitudes even into a lead segment of the nanotube are likely to be different.

Finally, we note that different coupling asymmetries (strong-weak, equal and weak-strong) of the two states have been observed in experiments (*e.g.* [3]), and the phase factor is therefore necessary to capture these result. Just as $\Delta_{KK'}$ varies between different shells, its phase seems to vary as well, *i.e.*, both the magnitude and the phase of the orbital coupling are fitting parameters of a nanotube shell.

# Single particle two-shell model and fRG

The fitting to the cotunneling spectroscopy in Figs. 3(b,e,f) is based on a single particle (minimal) model including two nanotube shells in the valence band. The Hamiltonian consists of two parts $H = H_0 + H_{B_{||}}$, where the first term includes spin-orbit interaction and intra/inter shell orbital coupling, while the second term accounts for the $B_{||}$ dependence. Noting that the Hamiltonian is spin-conserving makes it convenient to separate the $8\times 8$-matrix into two $4\times 4$ blocks. In the basis $\{|1K\sigma\rangle,|1K'\sigma\rangle,|2K\sigma\rangle,|2K'\sigma\rangle\}$ ($\sigma = \{\uparrow,\downarrow\} \mathrel{\widehat{=}} \{1,-1\}$), the blocks read

$$H_\sigma = \frac{1}{2}\begin{bmatrix} \sigma\Delta_{SO} & \Delta_{KK'1} & 0 & \Delta_{KK'12} \\ \Delta^*_{KK'1} & -\sigma\Delta_{SO} & \Delta^*_{KK'12} & 0 \\ 0 & \Delta_{KK'12} & 2\Delta E + \sigma\Delta_{SO} & \Delta_{KK'2} \\ \Delta^*_{KK'12} & 0 & \Delta^*_{KK'2} & 2\Delta E - \sigma\Delta_{SO} \end{bmatrix}$$

$$+\mu_B B_{||}\begin{bmatrix} g_{orb}+\sigma & 0 & 0 & 0 \\ 0 & -g_{orb}+\sigma & 0 & 0 \\ 0 & 0 & g_{orb}+\sigma & 0 \\ 0 & 0 & 0 & -g_{orb}+\sigma \end{bmatrix} \tag{15}$$

where $E_1$ mentioned in the article is chosen to be the zero of energy. These two $4 \times 4$ systems are diagonalized numerically and the resulting eigenvalues and eigenvectors can be used in subsequent calculations. We note that the intra-shell and inter-shell orbital couplings ($\Delta_{KK'1}$, $\Delta_{KK'2}$ and $\Delta_{KK'12}$) have phases $\phi_1$, $\phi_2$ and $\phi_{12}$.

The magnetic field dependence of the spectrum is shown in Fig. 3(a). In Fig. 1(c) the inter-shell orbital coupling $\Delta_{\mathrm{KK'12}}$ and the spin-orbit coupling $\Delta_{\mathrm{SO}}$ are set to zero and only one shell is shown. The parameters of Fig. 3(a) are given in the caption. Furthermore the eigenvectores are used to calculate the (magnetic field dependent) tunnel couplings (Fig. 3(d)) to the eigenstates as outlined for the spinless model. Most importantly for the description of the experimental data, the obtained spectrum of the quantum dot allows fitting the cotunneling spectroscopy data to extract the single particle parameters of the system. The cotunneling lines in Fig. 3(b,e,f) are thus found by calculating the energy difference to excited states from the ground state using the single particle energy spectrum in Fig. 3(a). Note, that the tunnel couplings are defined as $\Gamma_i = \pi\rho|t_i|^2$, where $\rho$ is the density of states in the leads.

In order to find a minimal model to describe the linear conductance of Fig. 3(c) we discard both the two highest and two lowest eigenenergies as well as their tunnel couplings (see below for further discussion). The remaining four levels in Fig. 3(a) - together with the gate voltage - and their tunnel couplings (all calculated with the extracted single particle parameters) are used as input for an fRG calculation [4]. Assuming an equal charging energy $U_c$ between all energy levels then yields the static Matsubara self energy including two-particle vertex corrections at $T = 0$, which in turn can be used to obtain the linear conductance (see Fig. 3(g)) via the Landauer-Büttiker formalism [4].

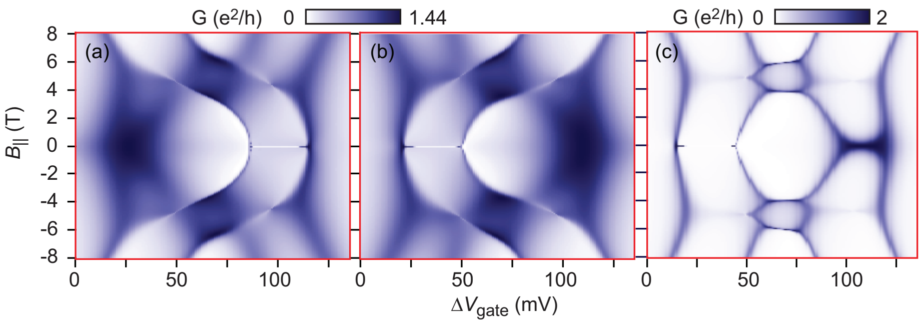


Figure S1: (a) Linear conductance for $\phi_{1/2} = 0.15\pi$. (b) Linear conductance for reversed shell asymmetry. (c) Linear conductance showing the level structure for $\Gamma_{1/2}^{L/R} = 0.09\,\mathrm{meV}$.

The fRG is a very flexible tool that allows to include and vary all essential single particle properties (as well as two-particle interactions), such as magnetic fields and spin-orbit interaction terms as well as complex tunnel couplings. This gives the opportunity to explore the parameter space (four initial tunnel couplings, one phase for the intra-orbital couplings and one phase for the inter-orbital coupling) in order to learn about the underlying physics. As a simple example consider the same parameters as in Fig. 3(g) but changing the phase from $\phi_{1/2} = 0.85\pi$ to $\phi_{1/2} = 0.15\pi$ (and $\phi_{12} = \pi$) leading to the expected reversal of the strong/weak Kondo-plateau position - see Fig. S1(a).[2] The plot also reveals that the slopes of the finite field Kondo ridges are slightly modified relative to those of Fig. 3(g). This effect primarily stems from the different choice of $\phi_{12}$, and this parameter can therefore be used to slightly tune the slopes.

A more interesting picture arises if one again takes the same parameters as in Fig. 3(g) (except $\phi_{12} = \pi$) but reverses the tunnel couplings for the shells, i.e. $\Gamma_{1/2}^{L/R} \to \Gamma_{2/1}^{L/R}$ - see Fig. S1(b). In this case the finite field Kondo ridges slant in the opposite direction which is less obvious based solely on the above two-shell model. This emphasizes the importance of being able to systematically investigate the parameter space in order to reproduce the interesting experimental features (strong/weak Kondo, slanted finite field resonance).

This leads to another observation: the correct sloping of the finite field Kondo ridges was reproduced only for those sets of tunnel-coupling parameters for which the lower shell was more strongly coupled than the higher shell - as it is often seen in carbon nanotubes (see e.g. the hole side of Fig. 1(c) in [5]). This leads us to conclude that the tunnel coupling to the shells (at zero field) has to decrease monotonically with increasing shell number in order to describe the experimental data in Fig. 3(a) where all slopes have the same direction.

Finally, we show that the single particle spectrum is indeed underlying the complex structure seen in Figs. S1(a-b) by plotting the conductance for a weakly

[2] The subscript of $\phi_{1/2}$ should be understood as $\phi_i$, $i = 1, 2$.

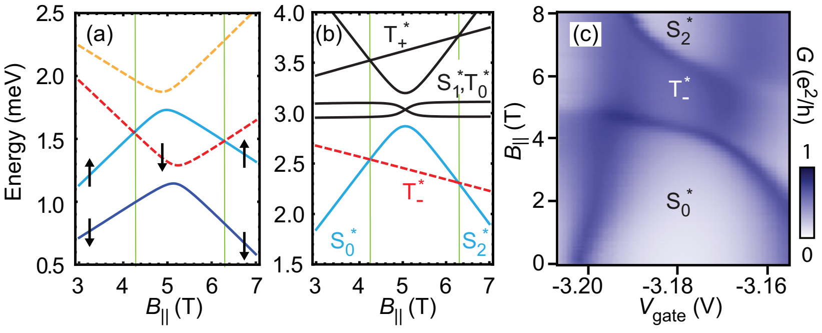


Figure S2: (a) Single particle spectrum of the inner four levels for N=4. (b) Singlet-triplet energy diagram obtained by adding the energies of the possible combinations of filling two electrons into the four states in (a). The two-electron states are not conventional singlets and triplets (denoted by the asterisk) due to the orbital component and spin-orbit interaction. Due to singlet-triplet crossings (lower two states) Kondo ridges are observed at finite magnetic field. (c) Linear conductance versus parallel magnetic field and gate voltage with the ground state marked in different regions. A gate voltage controlled spin ground state transition is realized at magnetic fields, where the Kondo ridges has a slope. The slope stems from different tunnel couplings of the involved singlet and triplet states (see e.g. Fig. S3(a-d)).

and equally coupled quantum dot (remaining parameters as in Fig. 3(g) except $\phi_{12} = \pi$) - see Fig. S1(c). This is exactly what would be expected using the single particle spectrum of Fig. 3(a) in the Letter, inserting the Coulomb energy by hand (separating each ground state charge transition).

## Detailed comparison between experiment and theory

The two-shell model presented in the Letter focuses on the behavior of the inner four states and their couplings (minimal model). This is primarily due to the interesting level crossing and anticrossing behavior at finite magnetic fields, which are shown to strongly modify the tunnel couplings. Furthermore, since inter-shell anticrossings with additional higher and lower shells are not taken into account, the couplings of the remaining upper and lower doublets (dashed blue/cyan and solid orange/yellow lines in Fig. 3(a,d)) are not correctly modeled.

The finite field level crossings in Fig. 3(a) leads to singlet-triplet Kondo ridges for $N = 4$ electrons as depicted in Fig. S2(a-c) (also observed for $N = 0$ and $N = 8$). In the experiment the ridges have a slope, which is reproduced in the theory plot of Fig. 3(g) due to different couplings of the states involved (and renormalization effects). The inter-shell orbital coupling phase $\phi_{12}$ is chosen to 0 to model the weakly ($B_{||} \sim \pm 3.8\,\mathrm{T}$) and strongly sloping ($B_{||} \sim \pm 7\,\mathrm{T}$) Kondo ridges seen in the experiment. The theory plot in Fig. 3(g) also nicely

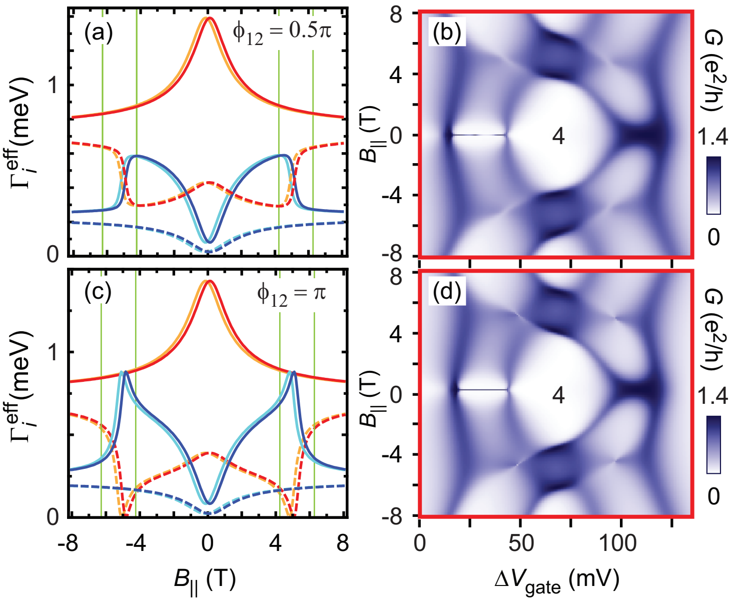


Figure S3: (a-b) Tunnel couplings versus $B_{||}$ and fRG linear conductance calculation versus $B_{||}$ and gate voltage. Parameters are the same as in Fig. 3(g) except the inter-shell orbital coupling phase $\phi_{12} = 0.5\pi$. (c-d) Same as (a-b) with $\phi_{12} = \pi$. The slopes of the Kondo ridges depend on the tunnel coupling difference at the respective level crossings (vertical green lines).

reproduces that the Coulomb peak to the right of the $N = 4$ valley continuously merges into the Kondo ridge - an effect not expected from the single particle picture. The crossover of the couplings related to the two inner doublets (solid blue/cyan and dashed orange/yellow lines in Fig. 3(a,d)) show a qualitative agreement between theory and experiments for $\phi_{12} = 0$ as mentioned in the Letter. It is, however, seen to be theoretically underestimated in Fig. 3(d) compared to the experiment: the solid blue/cyan and orange/yellow lines in Fig. 3(d) just cross each other compared to Fig. 3(c), where the narrow and broad Coulomb peaks interchange widths as the field is increased. This feature can be more accurately captured by choosing a different inter-shell orbital coupling phase (e.g. $\phi_{12} = \pi$), unfortunately, making the finite field sloping Kondo ridges less different. Figures S3(a-d) show the single particle tunnel couplings and linear conductance versus parallel field and gate voltage for two different phases $\phi_{12} = 0.5\pi$ and $\phi_{12} = \pi$. Tuning the phase from 0 to $\pi$ changes a minimum (maximum) of the couplings to a maximum (minimum) at the field corresponding to the anticrossings (compare Figs. 3(d) and S3(a,c)). Obtaining a complete quantitative agreement between theory and experiment for all features is thus difficult, and in the Letter we choose parameters for which the slope of the

Kondo ridges matches the experiment best. We note that one should be careful comparing the single particle couplings directly to the experiment, since tunnel couplings also may be renormalized. It is thus more correct to compare the experiment to the full fRG result in Fig. 3(g).

We next discuss the couplings of the remaining four states (solid orange/yellow and dashed blue/cyan lines in Fig. 3(a,d)). It is important to realize that the couplings in Fig. 3(d) do not reproduce the crossings of the couplings within a shell, inconsistent with the discussion in Fig. 2, i.e., no crossings are seen between the solid blue/cyan and the solid orange/red lines (similarly no crossings are observed for the dashed lines). These crossing can, however, be modeled by including the level anticrossing with the higher (shell 3) and the lower lying shell (shell 0) also observed in the experiment. The crossings of the couplings within shell 1 and 2 are then obtained by having inter-shell orbital couplings $\Delta_{KK'01}$ and $\Delta_{KK'23}$ with phases $\phi_{01} = \phi_{23} = \pi$. The solid orange/yellow lines thus drops to zero at magnetic fields corresponding to the anticrossings giving rise to a crossing of couplings between the solid blue/cyan and solid orange/yellow lines (similar argument is true for the shell related to the dashed lines).

The model thus gives a qualitative understanding of the observed data, and emphasizes that orbital disorder may modify the tunnel couplings.

## Peak fittings and tunnel coupling estimates

The tunnel couplings extracted in Fig. 2(d) are obtained by fitting the Coulomb peaks according to the procedure described in details in the supporting information of Ref. 15: the doublet tunnel coupling related to e.g. the ground state doublet is found by fitting only the even occupation sides of the Coulomb peaks in order to minimize the effect of Kondo correlations. The error bar indicates that the two Coulomb peak widths related to transport through the doublet experimentally are not the same. We acknowledge, that Kondo correlations still present at zero and even larger magnetic fields make an exact estimate difficult (as is generally the case in this regime), but we do believe that the extracted tunnel couplings do represent the qualitative tunnel coupling behavior of the doublets (also seen in colorscale plot of Fig. 1(b)).

# Tunneling-induced level shifts

The tunneling induced level shifts giving rise to the gate-dependence of the onset of inelastic cotunneling [3] is schematically explained in Fig. S4 for one electron in a shell with two energetically split doublets (red and blue levels). The width of the levels illustrates the coupling strength to the leads with the broader level having the strongest coupling, *i.e.*, the red level is strongest coupled. The level shifts are due to charge fluctuations which are most pronounced close to the Coulomb peaks of the one electron Coulomb diamond (see S4(g)).

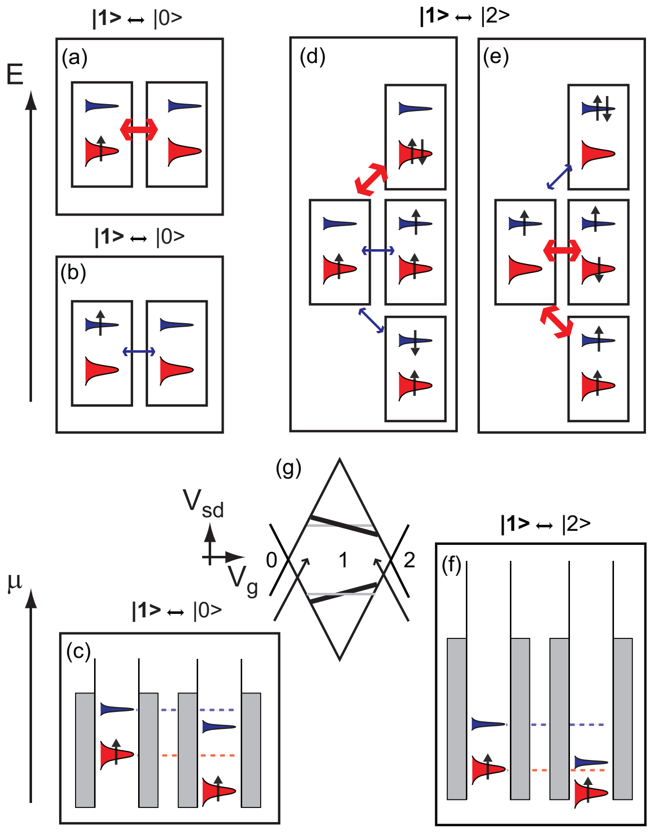


Figure S4: (a-b) Charge fluctuations from the one electron charge states via the zero electron charge state relevant in the left side of the Coulomb diamond leading to a larger doublet energy splitting as shown in (c). (d-e) Charge fluctuations from the one electron charge state to the two electron charge state via the empty states giving rise to smaller doublet splitting as shown in (f). (g) Schematics of the gate-dependent inelastic cotunneling onset due to tunneling-induced level shifts.

In the left side of the Coulomb diamond the electron may cotunnel out to the leads and back to the level, while an additional electron may tunnel onto the dot in the right side. The tunneling is accompanied with a correction to the energy lowering the energy of the states, *i.e.*, stronger tunneling leads to a larger correction. Figures S4(a-b) show the transitions possible between the one $|1\rangle$ and zero $|0\rangle$ electron charge states. For the weakly coupled level (b), the charge fluctuations (cotunneling events) are smaller than for the strongly coupled level, which therefore leads to a large/small energy shift of the strongly/weakly coupled level as shown in Fig. S4(c) (note, that the levels depicted in (c,f) are the related electrochemical potentials in a quantum dot energy diagram). The resulting spacing between the levels is thus larger and inelastic cotunneling occurs at a larger bias voltage.

In the right side of the Coulomb diamond, charge fluctuations occur via the two electron charge state $|2\rangle$ as shown schematically in Figs. S4(d-e). The level shift of the strongly/weakly coupled level will in this case (relatively) be small/large since there are two possibilities for tunneling via the strongly coupled levels in case of the weakly coupled level (see (e)). Thus the doublet splitting becomes smaller, when the energy corrections are taken into account as shown in Fig. S4(f). The resulting onset of inelastic cotunneling is seen in Fig. S4(g). Note that in the left/right side of the Coulomb diamond, the tunneling-induced level shift occurs via the filled/empty states in the quantum dot. Using this schematics it can also be understood that, for equal tunnel couplings of the doublets the level shifts are identical. Thus the onset of inelastic cotunneling occurs at the same bias voltage for all gate voltages as shown in the article in Fig. 2c, where the couplings are equal. This phenomenon has been thoroughly addressed in Ref. [3].

The origin of the sloping finite field Kondo ridges (Fig. 3(c,g)) can be understood in a similar manner. As seen in Fig. 3(a,d), the states (singlet and triplet) related to the Kondo effect have similar and different couplings to the leads at the two level crossings, respectively. This gives rise to weak and strong level renormalization, which can be compensated by applying a parallel magnetic field. The slope of the ridges can thus be predicted using the same simple picture to describe renormalization effects as explained above.

# References


[1] D. V. Bulaev, B. Trauzettel, and D. Loss, Phys. Rev. B **77**, 235301 (2008).

[2] S. Weiss, *et al.*, Phys. Rev. B **82**, 165427 (2010).

[3] J. V. Holm, *et al.*, Phys. Rev. B **77**, 161406 (2008).

[4] C. Karrasch, T. Enss, and V. Meden, Phys. Rev. B **73**, 235337 (2006).

[5] J. Cao, Q. Wang, and H. Dai, Nature Materials **4** (2005).
